# Supplementary material for: Tuning of topological properties in the strongly correlated antiferromagnet Mn$_3$Sn via Fe doping
Source: arXiv:2210.14150 source file (2022-10-25)
Supplement: Supplementary file 1 [file Supplemental_Material.pdf]

**Supplementary information**

# Tuning of topological properties in the strongly correlated antiferromagnet $Mn_3Sn$ via Fe doping

**Achintya Low, Susanta Ghosh, Susmita Changdar, Sayan Routh, Shubham Purwar, and S. Thirupathaiah***

Department of Condensed Matter and Materials Physics,

S. N. Bose National Centre for Basic Sciences, Kolkata, West Bengal-700106, India.

*setti@bose.res.in

## 1. Crystal and magnetic structures of $Mn_3Sn$

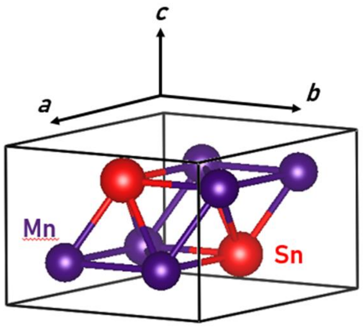


*Fig 1: Crystal structure of $Mn_3Sn$*

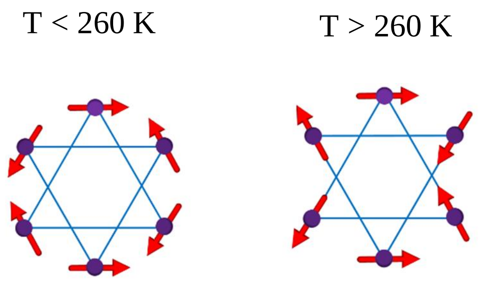


*Fig 2: (Left) spiral spin structure of $Mn_3Sn$ below 260K and (right) inverse triangular spin structure above 260 K*

Crystal structure of $Mn_3Sn$ is shown in figure 1. Hexagonal unit cell of $Mn_3Sn$ is formed with 6 Mn atoms and 2 Sn atoms in a kagome network (ab plane) of the crystal. The individual Mn magnetic moments form an inverse chiral spin structure [1] as shown right image of Fig 2 stabilized by DM interaction where the left panel in figure 2 represents the spiral or helical magnetic ordering [2,3] formed by the Mn atoms below transition temperature $T_{SR}$=260K.

## 2. Resistivity upturn fitting for $Mn_{2.65}Fe_{0.35}Sn$

There are different mechanisms to explain the low temperature resistivity upturn, (a) weak localization effect, in which mobile electrons scatter with impurity atoms and due to constructive quantum interference the resistivity minima is observed [4], (b) Kondo effect, in which scattering of conduction electrons with magnetic impurities results upturn in the resistivity [5], and (c) elastic electron-electron interaction in the presence of strong chemical or magnetic disorder [6, 7], leading to resistivity minima. Here, weak localization effect can be easily eliminated as we found the resistivity minima at relatively higher temperature of 50 K, whereas weak localization usually occurs at very low temperature [8, 9]. So, we tried to fit our resistivity data with Kondo and elastic electron-electron interaction formulae. The Kondo effect can be expressed as $\rho(T) = \rho_0 - Aln(T) + \beta T^p$ [5, 7], where $\rho_0$ is residual resistivity, middle term represents Kondo effect, and the last term represents inelastic electron-electron, electron-phonon, and electron-magnon scattering. In Fig. 3(a) we showed the fitted data overlapped on the original data and we clearly see a mismatch between the two curves. By considering only the elastic electron-electron scattering which can be expressed as $\rho = \rho_0 - \alpha T^{-\frac{1}{2}} + \beta T^P$[7], we fitted the data perfectly up to 100K and as can be seen from Fig. 3(b). The fitted parameters are $\rho_0 = 0.0059939 \pm 1.33\,e-06$ Ohm-cm, $\alpha = 1.489\,e-05 \pm 4.38\,e-07$ Ohm-cm, $\beta = 6.926\,e-09 \pm 2.45\,e-09$ Ohm-cm, and $p = 2.0937 \pm 0.0715$.

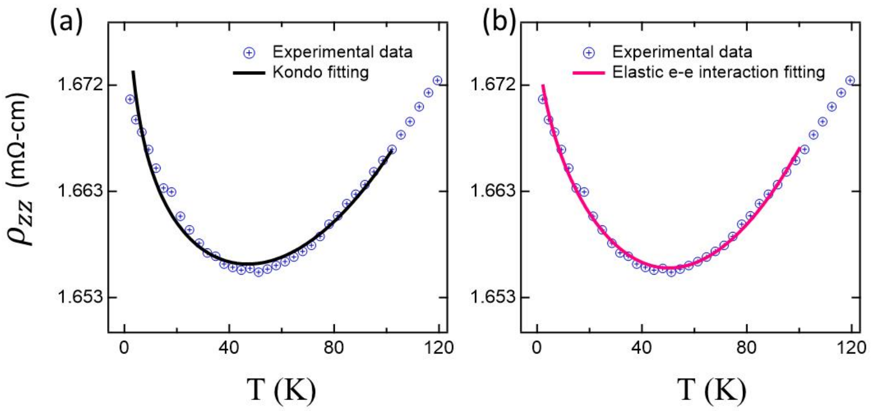


*Fig 3: Resistivity curve fitting of $Mn_{3-x}Fe_xSn$ for x=0.35 with two distinct formulism (a) Kondo effect and (b) elastic electron-electron interaction.*

## 3. Evolution of Magnetization M(H) Isotherms for *x*=0.25 and *x*=0.35

Field dependence of magnetization at different temperatures are shown in figures. 4 and 5. In Fig. 4, from $x = 0.25$, we see out-of-plane (H || z) magnetization varies almost linearly with field and with decreasing temperature a sigmoid-like ferromagnetic nature is growing. At 2 K, the out-of-plane magnetization dominates in-plane magnetization leading to magnetic anisotropy. Similarly, Fig. 5 represents

M(H) isotherms for $x = 0.35$ at various temperatures. We observe that the out-of-plane ferromagnetism (H || z) is stronger in $x$=0.35 compared to $x$=0.25 at 2 K.

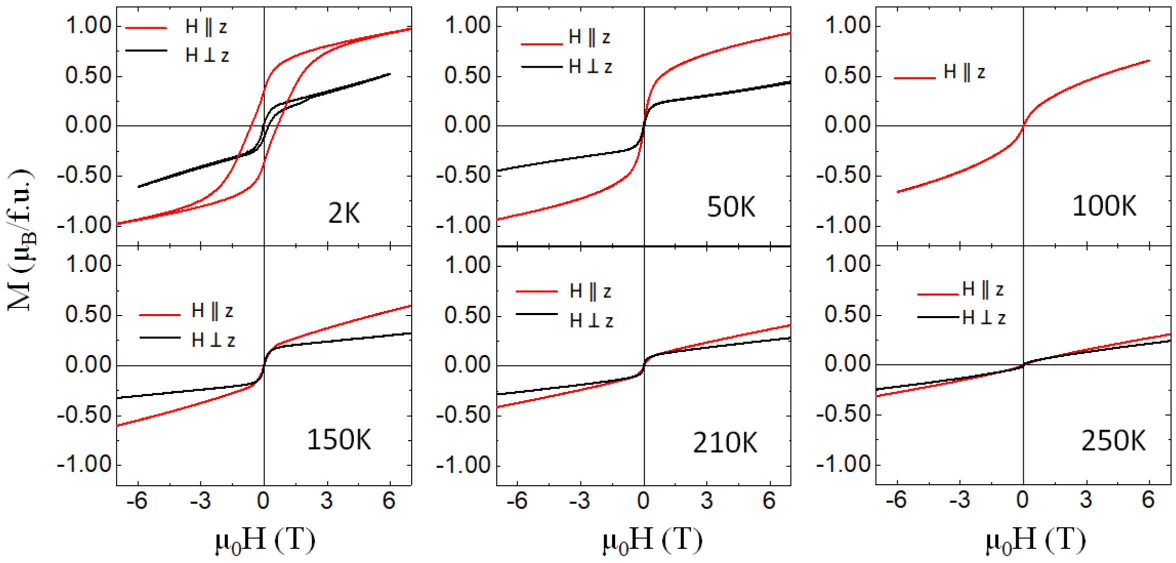


*Fig 4: Magnetization M(H) isotherms from $Mn_{3-x}Fe_xSn$ (x=0.25)*

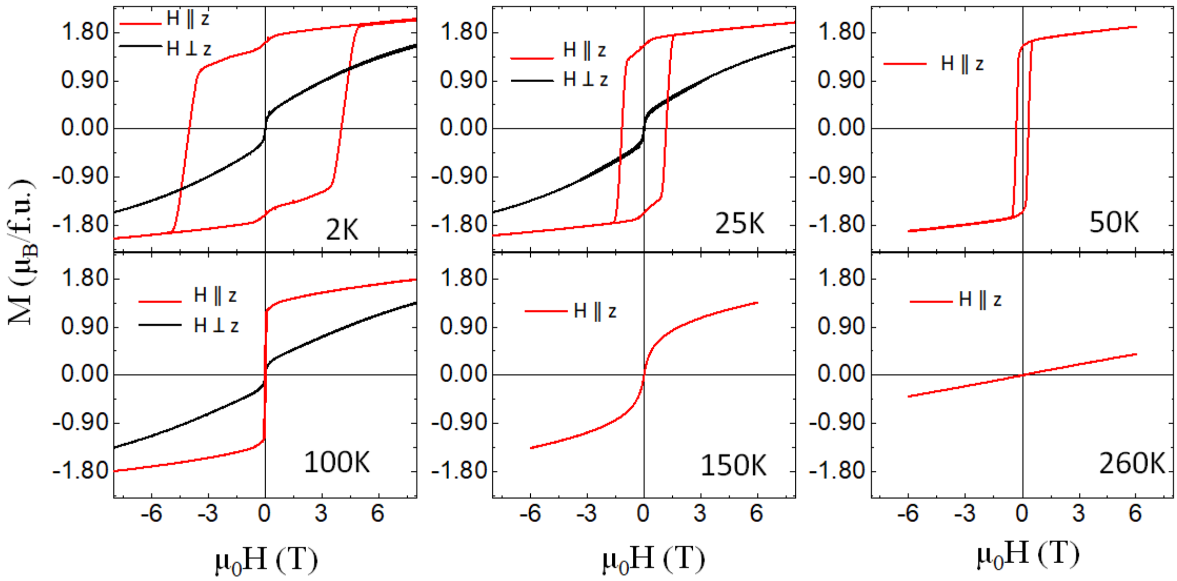


*Fig 5: Magnetization M(H) isotherms from $Mn_{3-x}Fe_xSn$ (x=0.35)*

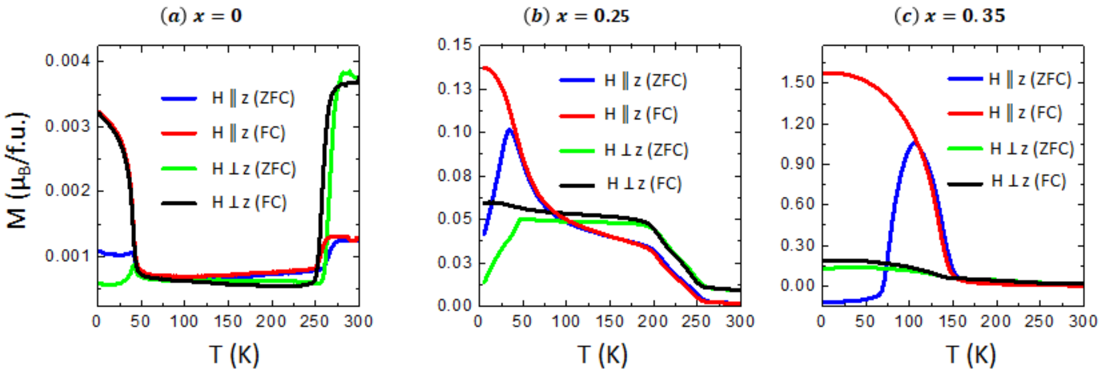


*Fig. 6: M(T) of (a) x=0, (b) x=0.25, and (c) x=0.35.*

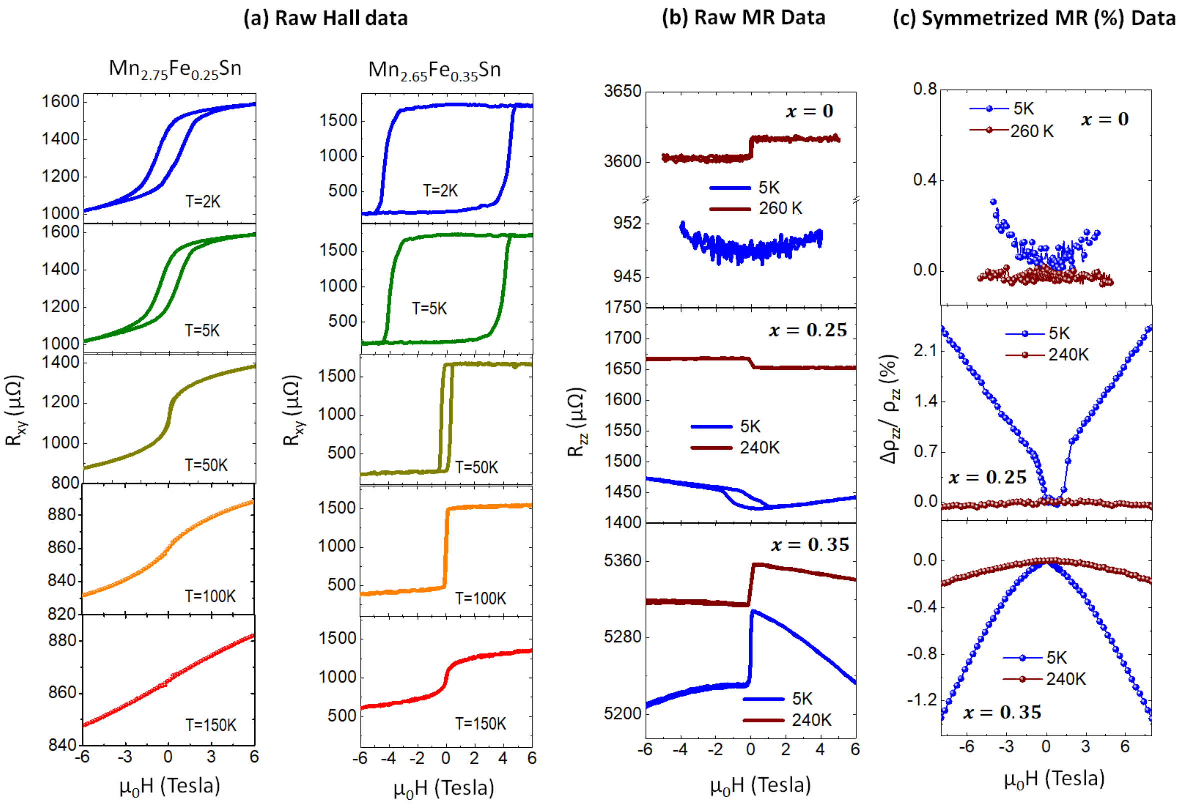


*Fig 7: (a) Raw Hall data of x=0.25 and x=0.35. (b) Raw MR data. (c) Symmetrised MR (%) data.*

# References:


1. T. Nagamiya, S. Tomiyoshi, and Y. Yamaguchi, Triangular spin configuration and weak ferromagnetism of $Mn_3Sn$ and $Mn_3Ge$, Solid State Communications **42**, 385 (1982).
2. J. Cable, N. Wakabayashi, and P. Radhakrishna, A neutron study of the magnetic structure of $Mn_3Sn$, Solid state communications **88**, 161 (1993).
3. T. Duan, W. Ren, W. Liu, S. Li, W. Liu, and Z. Zhang, Magnetic anisotropy of single crystalline $Mn_3Sn$ in triangular and helix-phase states, Applied Physics Letters **107**, 082403 (2015).

4. B. L. Altshuler, D. Khmel'nitzkii, A. I. Larkin, and P. A. Lee, Magnetoresistance and hall effect in a disordered two-dimensional electron gas, Phys. Rev. B **22**, 5142 (1980).
5. J. Kondo, Resistance minimum in dilute magnetic alloys, Progress of theoretical physics **32**, 37 (1964).
6. P. A. Lee and T. Ramakrishnan, disordered electronic systems, Reviews of modern physics **57**, 287 (1985).
7. S. Dhara, R. R. Chowdhury, and B. Bandyopadhyay, Observation of resistivity minimum at low temperature in $Co_xCu_{1-x}$ (x=0.17–0.76) nanostructured granular alloys, Physical Review B **93**, 214413 (2016).
8. Lu, Hai-Zhou, and Shun-Qing Shen. "Weak localization and weak anti-localization in topological insulators." *Spintronics Vii*. Vol. 9167. SPIE, 2014.
9. Xu, Yan, et al. "Low-temperature resistivity minimum and weak spin disorder of polycrystalline $La_{2/3}Ca_{1/3}MnO_3$ in a magnetic field." *Physical Review B* **73**, 22 (2006): 224410.
